# Supplementary material for: Hydrogenic Spin-Valley states of the Bromine donor in 2H-MoTe$_2$
Source: arXiv:2305.00719 source file (2023-05-01)
Supplement: Supplementary file 1 [file MoTe_2_Br_SI.pdf]

# Supplementary : Hydrogenic Spin-Valley states in Bromine-doped 2H-$MoTe_2$

Valeria Sheina[1], Guillaume Lang[2], Vasily Stolyarov[3,4], Vyacheslav Marchenkov[5], Sergey Naumov[5], Alexandra Perevalova[5], Jean-Christophe Girard[1], Guillemin Rodary[1], Christophe David[1], Leonnel Romuald Sop[1], Debora Pierucci[1], Abdelkarim Ouerghi[1], Jean-Louis Cantin[6], Brigitte Leridon[2], Mahdi Ghorbani-Asl[7], Arkady V. Krasheninnikov[7,8] and Hervé Aubin[1]

[1]Centre de Nanosciences et de Nanotechnologies (C2N), UMR CNRS 9001, Université Paris-Saclay, 10 Boulevard Thomas Gobert, Palaiseau, 91120, France.
[2]Laboratoire de Physique et d'Étude des Matériaux, UMR CNRS 8213, ESPCI Paris, Université PSL, Sorbonne Université, 10 Rue Vauquelin, Paris, 75005, France.
[3]Advanced Mesoscience and Nanotechnology Centre, Moscow Institute of Physics and Technology, Dolgoprudny, 141700, Russia.
[4]Advanced Mesoscience and Nanotechnology Centre, National University of Science and Technology MISIS, Moscow, 119049, Russia.
[5]M.N. Mikheev Institute of Metal Physics, UB RAS, Ekaterinburg, 620108, Russia.
[6]Institut des NanoSciences de Paris, UMR CNRS 7588, Sorbonne Université, 4 Place Jussieu, Paris, 75005, France.
[7]Institute of Ion Beam Physics and Materials Research, Helmholtz-Zentrum Dresden-Rossendorf, Dresden, 01328, Germany.
[8]Department of Applied Physics, Aalto University, P.O. Box 11100, Aalto, 00076, Finland.

# 1 Group theory

Since the early work of Kohn and Luttinger [1], it is usual to describe the quantum states of shallow dopants on the basis of Bloch states. To do so, however, implies that some of the dopant orbitals be allowed to hybridize by symmetry to the Bloch states. This can be demonstrated rigorously using band representations theory, a theory of irreducible representations of space groups. To our knowledge, band representation theory applied to the impurity problem has been first discussed in Ref. [2]. Nowadays, band representations theory is essential for the classification/identification of materials with distinct topological properties [3] and online applications have been developed on the Bilbao crystallographic server [4, 5].

For an impurity center, band representation theory shows how the space group irreps restricts to the irreps of the site symmetry group. Reciprocally, it provides the space group irreps induced by the irreps of the site symmetry group. Using the application DSITESYM [5] on the Bilbao server, we can show that the p orbitals of the Br atom, restricts to the double-group irreps $\bar{\mathrm{E}}_1$, $^1\bar{\mathrm{E}}$ and $^2\bar{\mathrm{E}}$ of the $\mathrm{C_{3v}}$ point-group, shown in table 1, induces the irreps (K8 to K12) and (LD3, LD4) of the group of the wavevector **K** and **Q**, respectively. The irreps (K8 to K12) corresponds to the valence and conduction bands at the **K**-point and the irreps corresponds to the conduction bands (LD3, LD4) at the **Q**-point, as indicated in Fig. 1 of the main text. This implies that the p-orbitals of the Br atoms are allowed by symmetry to hybridize with the valley Bloch states. This is confirmed by DFT calculations [6] showing that both the $\mathrm{p}_x$,$\mathrm{p}_y$ orbitals and the $\mathrm{p}_z$ orbital of the anion contribute to the conduction band **Q**-valleys. Actually, the $\mathrm{p}_z$ orbital has its largest contribution at the **Q**-valleys and has zero contribution to the **K**-points of both the valence and conduction bands. However, the $\mathrm{p}_x$,$\mathrm{p}_y$-orbitals have also contributions to the **K**-points of both the valence and conduction bands.

Following the notations of Ref. [7], the character table of the point double-group $\mathrm{C_{3v}}$ is :

**Table 1 Character table of the $\mathrm{C_{3v}}$ double-group**

| $\mathrm{C_{3v}}$ | $E$ | $C_3^+$ | $C_3^-$ | $3\sigma_v$ | $\bar{E}$ | $\bar{C}_3^+$ | $\bar{C}_3^-$ | $3\bar{\sigma}_v$ |
|---|---|---|---|---|---|---|---|---|
| $A_1$ | 1 | 1 | 1 | 1 | 1 | 1 | 1 | 1 |
| $A_2$ | 1 | 1 | 1 | $-1$ | 1 | 1 | 1 | $-1$ |
| $^1E$ | 1 | $\omega$ | $\omega^*$ | 0 | 1 | $\omega$ | $\omega^*$ | 0 |
| $^2E$ | 1 | $\omega^*$ | $\omega$ | 0 | 1 | $\omega^*$ | $\omega$ | 0 |
| $^1E_{1/2}$ | 1 | $-\omega$ | $-\omega^*$ | 0 | $-1$ | $\omega$ | $\omega^*$ | 0 |
| $^2E_{1/2}$ | 1 | $-\omega^*$ | $-\omega$ | 0 | $-1$ | $\omega^*$ | $\omega$ | 0 |
| $^1E_{3/2}$ | 1 | $-1$ | $--1$ | $-1$ | $-1$ | 1 | 1 | 1 |
| $^2E_{3/2}$ | 1 | $-1$ | $-1$ | 1 | $-1$ | 1 | 1 | $-1$ |

# 2 Transport properties

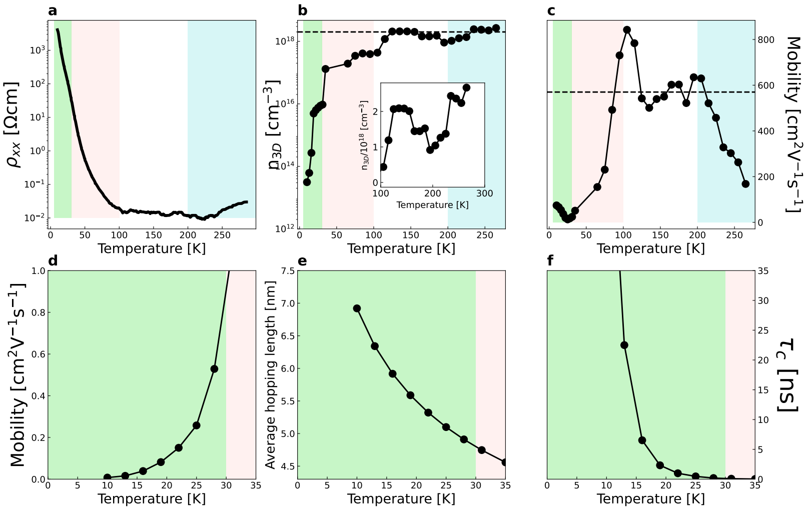


**Fig. 1 Transport properties of Br-doped 2H-MoTe$_2$** **a**, Longitudinal resistivity $\rho_{xx}$ as a function of temperature. It is calculated from $\rho_{xx} = R_{xx} l \times t/L$ where $t \approx 30$ $\mu$m is the thickness of the crystal, $l \approx 1$ mm the width and $L \approx 1$ mm the length. The room temperature resistivity is $\rho \approx 50$ $m\Omega$ $cm$ and decreases upon cooling down to the temperature of 225 K, indicating a saturation regime from room temperature down to 225 K where the mobility is limited by phonon-scattering. At lower temperature, an activated regime and a hopping regime are visualized on an Arrhenius plot as shown in main text. **b**, Carrier concentration $n_{3D}$ on semilog scale as a function of the temperature. From the transverse Hall resistance R$_{xy}$ measured as a function of a perpendicular magnetic field **B**, one obtains the Hall coefficient $\rho_H = \frac{R_{xy} t}{B}$ and so the carrier concentration from $n_{3D} = \frac{1}{e\rho_H}$. In the saturation regime, $n_{3D} = 2 \times 10^{18}$ cm$^{-3}$ as indicated by the horizontal dashed line. Inset: Carrier concentration as function of temperature on linear scale to highlight the temperature dependence from 150 K to 300 K. **c**, Mobility as function of temperature. The mobility is calculated from $\mu = 1/e\rho_{xx} n_{3D}$. Using the relation for the resistivity and the carrier concentration and using $l = L$, the mobility $\mu = R_{xy}/R_{xx}$ does not depend on geometrical factors and so is obtained with high precision. The mobility is increasing from room temperature down to 225 K because of the reduction in phonon scattering as expected in the saturation regime [8]. It reaches a maximum of $\mu \approx 570$ cm$^2$V$^{-1}$s$^{-1}$ as indicated by the horizontal dashed line. The peak in mobility just before the activated regime is commonly observed in doped semiconductors [8] because of the drop in carrier concentration at this temperature as visible on panel **b**. However, this peak and the mobility data at lower temperature are not meaningful. **d** Mobility in the hopping regime calculated from $\mu = 1/e\rho_{xx} n_{3D}$ where we assume that all carriers of density $n_{3D} = 2 \times 10^{18}$ cm$^{-3}$ are contributing to the hopping transport, as done in Ref. [8]. **e**, Hopping length calculated following Ref. [8]. The temperature dependence of the resistivity is fitted by a Mott law $\rho \propto \exp(\xi_c)$ with the correlation length $\xi_c = (T_0/T)^{1/3}$, valid at two dimensions, and gives $T_0 \approx 27 \times 10^3$ K. From the correlation length, one obtains the average hopping length $\bar{r} = a\xi_c/4$ where $a$ is the Bohr radius calculated in the main text. **f**, Correlation time $\tau_c$ calculated using the Einstein relation $\mu(T) = eD/k_B T$ between the mobility calculated in the hopping regime and the diffusion constant $D = \bar{r}^2/\tau_c$.

# 3 Fitting of the ESR data

The spectrum is constituted of a central line with additional sidelines and can be nicely described by an effective spin Hamiltonian assuming two different contributions of identical g-tensor. One contribution arises from electrons localized on single Br donors, i.e., not experiencing hopping, and produces the sidelines resulting from the hyperfine coupling of the electronic spin with the nuclear spin of the Br atom. The second contribution produces the central line and arises from the donor electrons hopping between different Br sites, with the hyperfine structure being suppressed due to the different nuclear spin polarizations probed by the electron spin. A similar model was employed for arsenic acceptors in MoS$_2$ [9].

To fit the experimental ESR data, we use the effective spin Hamiltonian:

$$\hat{\mathcal{H}} = \mu_B \hat{\vec{S}} \overleftrightarrow{g} \hat{\vec{B}} + \hat{\vec{S}}. \overleftrightarrow{A} . \hat{\vec{I}} + \hat{\vec{I}}. \overleftrightarrow{Q} . \hat{\vec{I}} \tag{1}$$

where $\hat{\vec{S}}$ is the electron spin 1/2, $\hat{\vec{I}}$ the nuclear spin 3/2, $\overleftrightarrow{g}$ is the g-factor tensor, $\overleftrightarrow{A}$ the hyperfine coupling tensor and $\overleftrightarrow{Q}$ the quadrupole coupling tensor written as :

$$\overleftrightarrow{Q} = \frac{h\nu_q}{4I(2I-1)} \begin{bmatrix} -(1-\eta) & & \\ & -(1+\eta) & \\ & & 2 \end{bmatrix} \tag{2}$$

where $\nu_q = e^2qQ/h$ is the quadrupole coupling constant in MHz and $\eta$ the quadrupolar asymmetry coefficient. The coupling constant depends on the nuclear quadrupole moment of bromine $Q = 0.3$ barn [10] and the electric field gradient e$q$. The quadrupolar coupling constant was also included to fit the ESR spectrum of As acceptors in MoS$_2$ [9].

We show now how to extract the values of the hyperfine and quadrupolar coupling constants directly from the experimental data. Figure 2a shows the effect of the hyperfine coupling between the S = 1/2 electron spin and the nuclear spin I = 3/2. Each of the two energy levels of the electron spin splits into four levels, one for each nuclear spin projection. This leads to four ESR resonance lines, as shown in Fig. 2b. Because the nuclear quadrupole moment aligns preferentially with the electric field gradient (EFG), this produces an anisotropy term for the nuclear spin, described by the tensor $\overleftrightarrow{Q}$. In this case, the energy levels with nuclear spins S = ±3/2 (S = ±1/2) shift to lower (higher) energy, as shown in Fig. 2c with magnetic field along the z direction (ie, the main axis of EFG). In this situation, four resonances lines are observed, as shown in Fig. 2d, and the presence of quadrupolar coupling is not directly visible. However, applying the magnetic field in-plane, Fig. 2f shows now three major lines because the states with $S = \pm 3/2$ nuclear projections have now identical energies, Fig. 2e. Furthermore, because of mixing between the nuclear spin states, transitions between states with different nuclear spin projection are now possible as indicated by vertical grey lines Fig. 2e, they give rise to ESR resonances of small amplitude as shown in Fig. 2f.

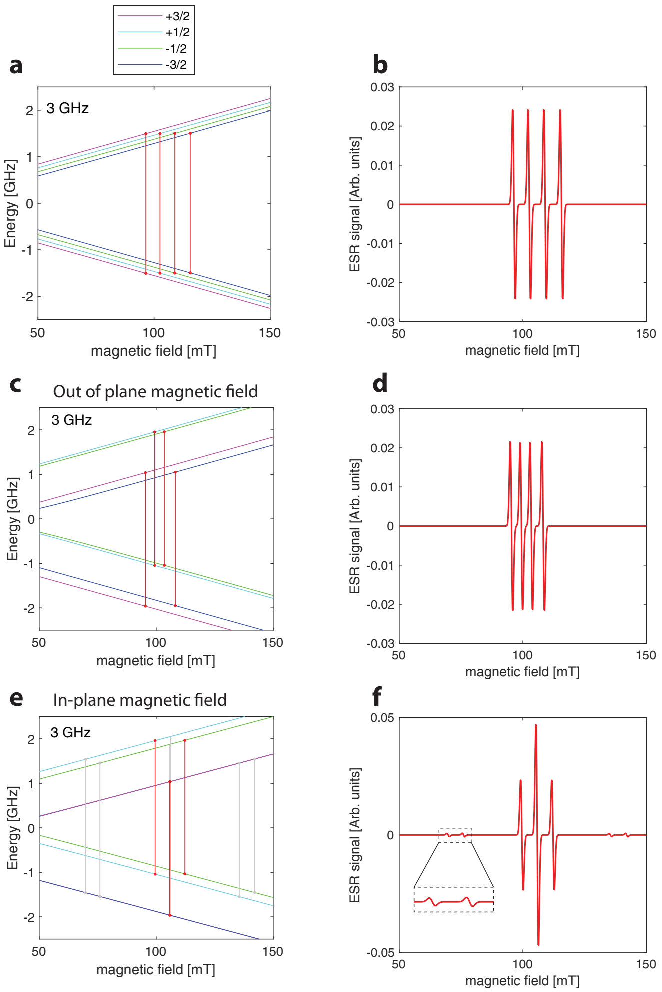


**Fig. 2 Simulation of the effect of hyperfine and quadrupolar coupling. ace** Energy levels of a spin system composed of an S=1/2 electron spin and I = 3/2 nuclear spin as function of magnetic field. Two sets of energy levels, symmetric with respect to the horizontal line of zero energy, correspond to the two electron spin projections $S = \pm 1/2$. The different line colors correspond to the different nuclear spin projections indicated in the legend. The vertical red and gray lines indicate allowed ESR transitions. The simulation have been performed for a 3 GHz microwave signal to make the energy differences between the energy levels visible on the plots. **a**, With hyperfine coupling only. **c**, With hyperfine and quadrupolar coupling constants where the magnetic field is applied along the z direction. **e**, With hyperfine and quadrupolar coupling constants where the magnetic field is applied in-plane. Note the presence of only three major resonance lines, red vertical lines, and four additional resonance lines, vertical gray lines, symmetrically located on both sides of the major resonances lines. **bdf**, Corresponding simulated resonance spectra. On panel **f**, note the presence of additional resonances lines, due to nuclear spin mixing, of small amplitude, also shown in the zoom-in insert.

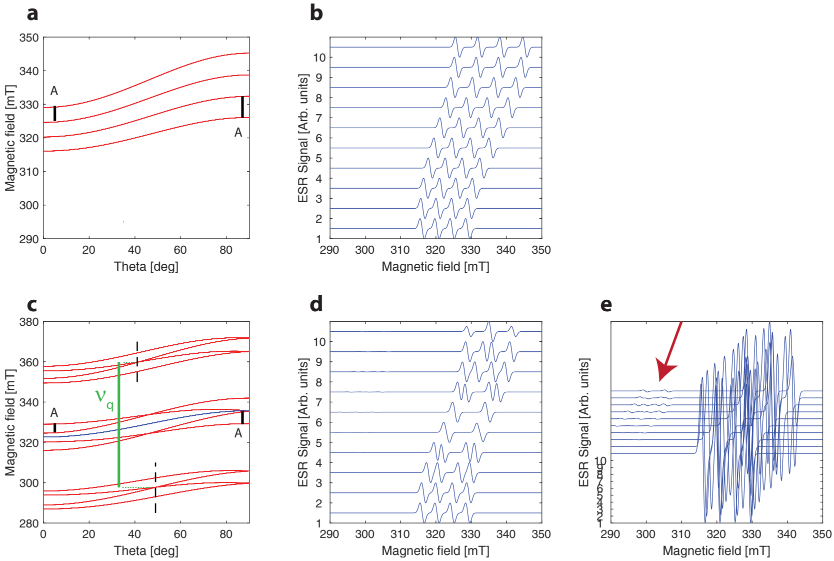


**Fig. 3 Angular dependence of simulated ESR signal.** Simulation of a spin system with a single electron S = 1/2 and a nuclear spin I = 3/2, using the g-factors and hyperfine parameters given in table 2, and the quadrupole constant $\nu_q = -1800$ MHz. The parameters are identical to those used for fitting the experimental data except that we did not include the contribution of the second S=1/2 electron to facilitate the visibility of multiple lines. The position of the resonance lines in mT as function of azimuthal angle $\theta$ where $\theta = 0$ corresponds to the magnetic field along the z-axis are shown **a** (**c**) in the absence (presence) of quadrupolar coupling. The vertical continuous black lines, labeled by A, indicate that the resonance separation is controlled by the hyperfin coupling constant. **c**, The vertical continuous green lines indicate that the separation between the three sets of lines is controlled by the quadrupole coupling constant $\nu_q = -1800$ MHz. The vertical black dashed lines indicate the weak quadrupole-induced resonances lines are most visible. **bde**, Corresponding resonances spectra as function of magnetic field. **e** Zoom on the data shown in panel **d** where the quadrupole-induced resonances, indicated by a red arrow, are visible.

The identification of the effects of quadrupolar coupling requires measurements of the ESR signal as function of orientation of magnetic field. Figure 3 shows the simulation of ESR spectra as function of azimuthal angle between the magnetic field vector and the z axis. In the absence of quadrupolar coupling, four resonances lines are observed at all angles, where the energy separation is controlled by the hyperfine coupling constant. In the presence of quadrupolar coupling, three sets of resonance lines are observed, separated by the value of the quadrupolar coupling constant. Within each set, two, three of four resonances lines are observed, separated at maximum by the hyperfine coupling constant. The central set is composed of major resonances of larger amplitude, the two lateral sets result from nuclear spin mixing and are of weak amplitude. At two particular angles, 41° and 49° in Fig. 3c, lines crossing is observed in the two lateral sets, where the resonance signals resulting from quadrupolar

coupling becomes most visible as shown in Fig. 3e. This quadrupolar-induced resonance peak is also visible in the experimental data as shown in Fig. 4a. Between 90 ° and 50 °, this peak is seen on one side, below 50 °, this peak is seen on the other side, symmetrically. We did not analyze more precisely the angular dependence of this quadrupolar-induced resonance line. As the separation between the two peaks corresponds to $\nu_q$ (see the simulation on Fig. 3c), the experimental data (Fig. 4b) yields the quadrupolar constant $\nu_q = e^2qQ/h = -1800$ MHz. Within this same angular range, 41° to 49°, we see on the simulation Fig. 3cd that the four major resonance lines from the central set merge into two resonances. On the experimental data, Fig. 4a, we see indeed that the hyperfine resonances are most resolved for in-plane and out-of plane magnetic field but in or close to the above angular range, only a broad peak is visible due to the large overlap of resonance lobes. In the absence of quadrupolar coupling, the visibility of the hyperfine lines should not change with angular orientation. Thus, two characteristics of the data, the apparition of peaks of weak amplitude symmetrically with respect to the major resonances lines and the angular dependence of the resolvability of the hyperfine lines, seems to be simply explained by the introduction of the quadrupole coupling constant. The amplitude of the two components, in-plane and out-of-plane, of the hyperfine coupling tensor are obtained from the separation between the hyperfine lines, as shown Fig. 4a.

**Table 2 Parameters of the effective spin Hamiltonian.**

| | **xx** | **yy** | **zz** |
|---|---|---|---|
| **g** | 2.0178 | 2.0178 | 2.0995 |
| **A** (MHz) | 180 | 180 | 127 |

Using the value $\nu_q = -1800$ MHz, $\eta = 0$ and the hyperfine and g-factor parameters summarized in table 2, the effective Hamiltonian is solved with Easyspin [11]. We find that best fitting is obtained using a weight of 0.01 for the first contribution, i.e., the electrons localized on single Br donors where the quadrupolar and hyperfine coupling are included, and using a weight of 0.99 for the second contribution, i.e., the electrons hopping between different Br sites for which the hyperfine structure is suppressed. We insist that the two contributions have identical g-factors and arise from the same electrons provided by the Br dopants as demonstrated by the angular dependence Fig. 4 which shows that the g-factor of both contributions, the central line and the sidelines, is changing identically with the angular orientation. A minimal MATLAB program to reproduce the fitted ESR line is joint as a supplementary file.

With those parameters, the experimental data with the fitting curves are shown as function of angle, Fig. 4a, and temperature, Fig. 5, where one can see

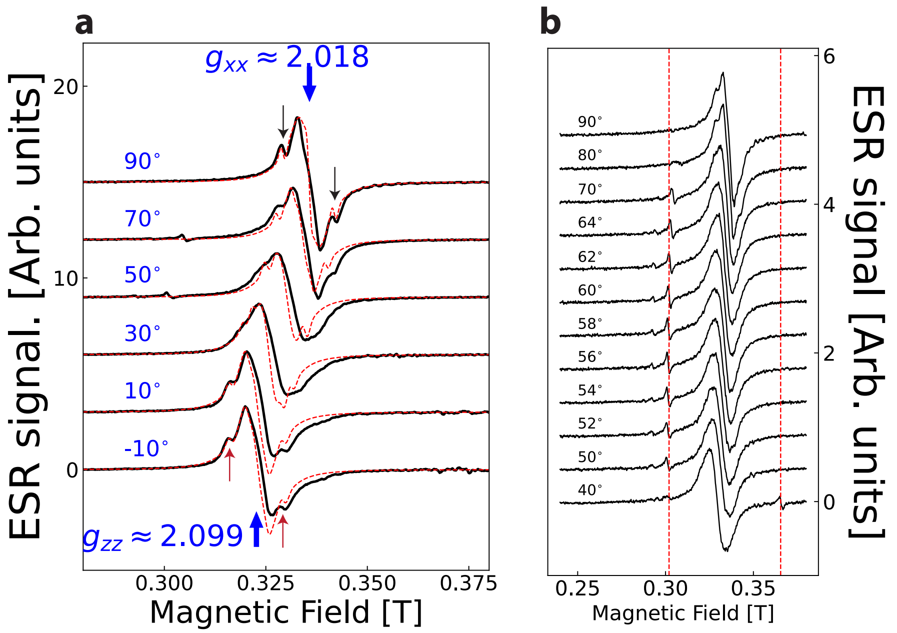


**Fig. 4 ESR signal as function of azimuthal angle. a**, The black curves show the ESR signal as function of azimuthal angle. The red dashed curves show the fitting curves. The red arrows are separated by 3 $\times A$, the black arrows are separated by 2 $\times A$, enabling the determination of the hyperfine coupling constants for in-plane and out-of-plane magnetic field. **b**, The black curves show the ESR signal as function of azimuthal angle near 50 ° where the quadrupolar-induced weak resonances are observed in the simulation. We see clearly, at 50 ° and 40 °, that the two weak resonances are located symmetrically with respect to the major line. From their magnetic field separation, indicated by vertical red dashed lines, the quadrupolar coupling constant $\nu_q = -1800$ MHz is determined.

that the model provides a reasonable fit of the experimental data. An interesting outcome of this analysis is the identification of the resonances resulting from the mixing of different nuclear spin states which allows to extract the quadrupole coupling constant $\nu_q = -1800$ MHz. This value is very large but comparable to the values of 577 MHz found for alkyl-Br molecules[12] and 832 MHz for $Br_2$ molecules[13, 14]. Ab-initio calculations of the quadrupole coupling constant[12] have shown that relativistic effect, i.e. spin-orbit coupling, leads to an increase of the quadrupole coupling constant. In 2H-$MoTe_2$, the large spin-orbit coupling could explain the enhanced quadrupole coupling constant. Further works is needed to confirm and analyze more precisely this phenomenon.

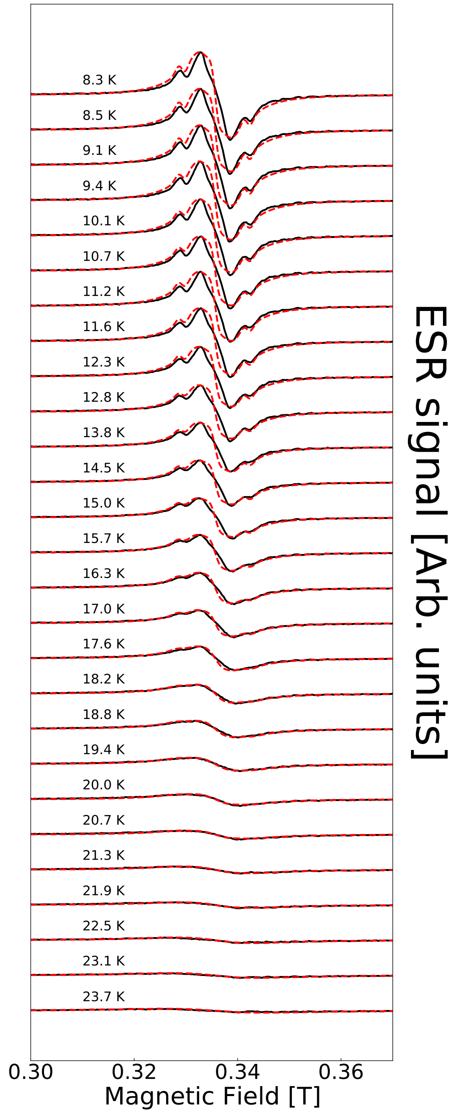


**Fig. 5 ESR signal as function of temperature.** The black curves show the ESR signal as function of temperature for a magnetic field applied in-plane. The red dashed curves show the fitting curves from which the linewidth and the spin coherence time is extracted as described in the main text.

# 4 Hyperfine-limited lifetime

In a quantum dot or hydrogenoic dopant, it has been established theoretically[15] that the hyperfine limited coherence time should increase with the number of atomic nucleus N explored by the electron as:

$$T_2^* = \hbar\sqrt{\frac{3N}{2\sum_j I_j(I_j+1)A_j^2 a_j}} \tag{3}$$

where $a_j$ is the natural abundance of the nucleus element j of spin $I_j$.

This formula was employed by Jiang et al.[16] to describe the hyperfin-limited coherence time of electron localized in $MoS_2$, which they found to be about 40 ns. Using this same formula, as well as more precise calculation adapted to TMDC by Wu et al.[17], we find that the hyperfine limited coherence time should be about 100 ns.

# 5 Additional STM images

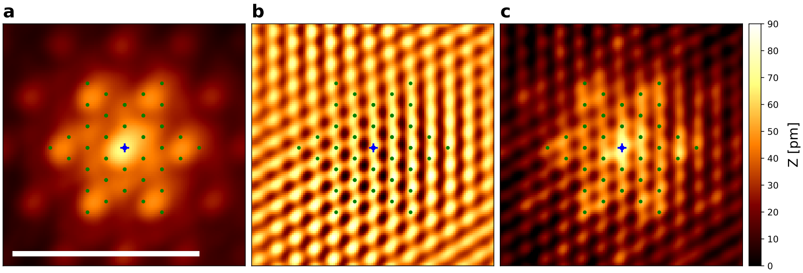


**Fig. 6 Atomic position of the Br dopant.** **a**, Topographic STM image of the Br$_{\mathrm{Te}}$ dopant. To locate its position with respect to the Te lattice, a 2D FFT is performed followed by a selection of the Bragg peaks and reversed FFT, whose results is shown in panel **b**, where the Te atom lattice is observed. This last image is multiplied by 200 and added to the original topographic image to highlight the position of the dopant with respect to the Te lattice, shown panel **c**. The Br$_{\mathrm{Te}}$ is clearly substituting a Te atom. A plus symbol on each image is plotted at the same position to help the visualization of the dopant position. The position of Te atoms is indicated as green on each image. The scale bar on panel **a** is 3 nm long.

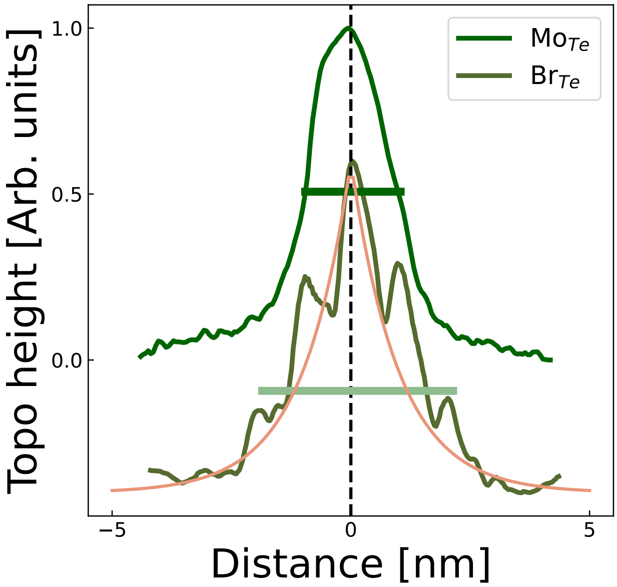


**Fig. 7 Topographic profile of the two point-defects.** The scale bars are 2 nm and 4 nm long for Mo$_{\mathrm{Te}}$ and Br$_{\mathrm{Te}}$, respectively. The continuous red curve is a plot of the envelope function $\rho(r) = |\psi(r)|^2 \propto \exp(-2r/a_B)$ where $\psi(r) \propto \exp(-r/a_B)$ describes the decay of the n = 1 hydrogenic wavefunction.

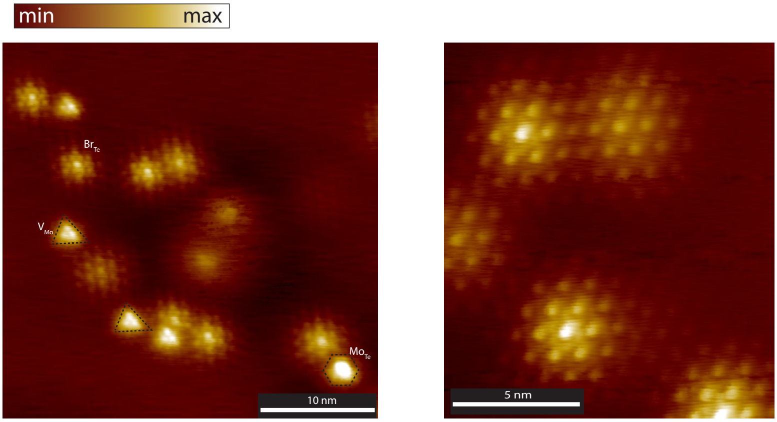


**Fig. 8 STM topography of the bromine-doped 2H-MoTe$_2$.** The topographies are taken at sample bias = -1 V and temperature T = 77 K. Left: Large scale STM topography showing multiple $Br_{Te}$ dopants, $Mo_{Te}$ antisites and $V_{Mo}$ vacancies. The white scale bar is 10 nm long. Right: Large scale STM topography showing 5 $Br_{Te}$ dopants. The white scale bar is 5 nm long.

From several large scale topographic maps such as shown in Fig. 8, the density of dopants and point-defects can be estimated, the values are given in the table below:

**Table 3 Point-defects densities.**

| | $V_{Mo}$ | $Mo_{Te}$ | $Br_{Te}$ |
|---|---|---|---|
| Density $[cm^{-2}]$ | $6.7 \times 10^{11}$ | $5 \times 10^{10}$ | $4 \times 10^{11}$ |

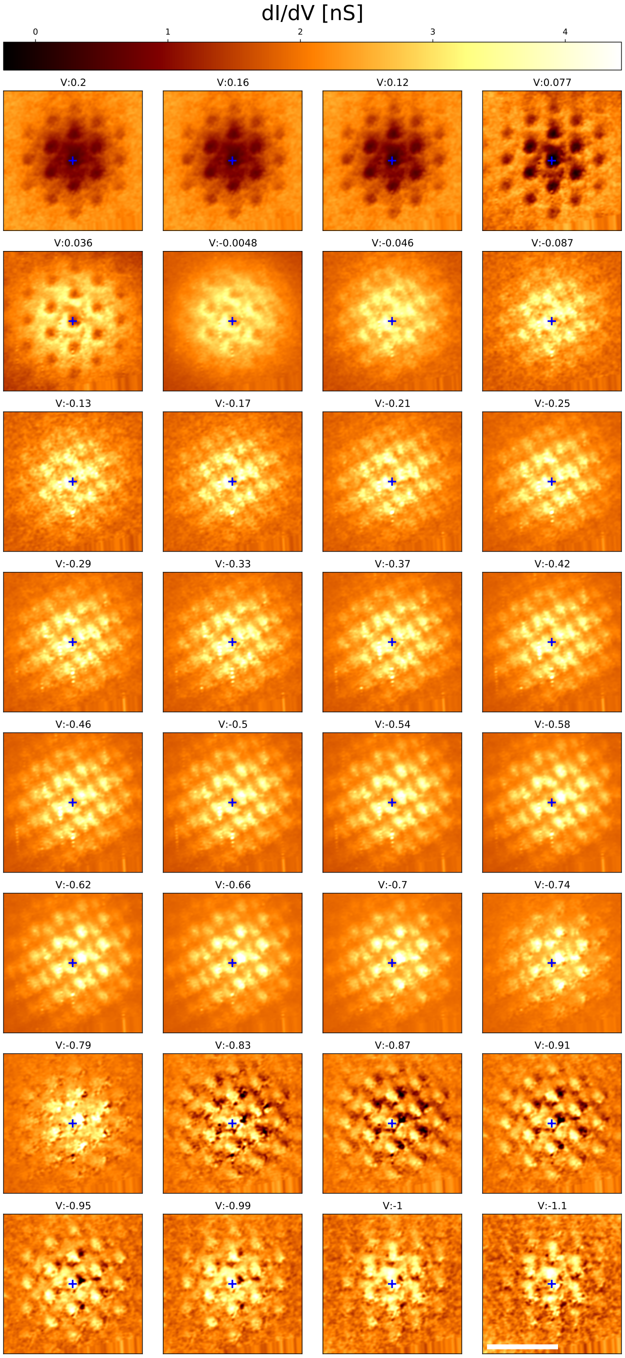


**Fig. 9 Conductance maps at different sample bias.** Differential conductance maps $\frac{\mathrm{d}I}{\mathrm{d}V}$ from the conduction band at sample bias = 0.2 V, to the valence band at sample bias = -1.1 V. The white scale bar on the last panel is 3 nm long. A plus symbol indicates the center of the images.

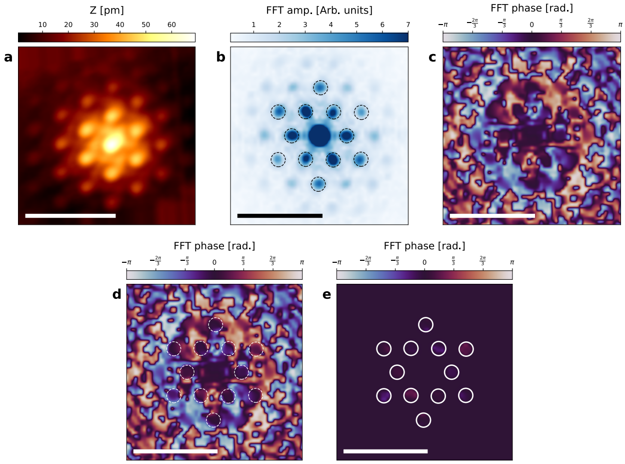


**Fig. 10 Displaying the phase of a 2D FFT.** The phase of the 2D-FFT is relevant only at wavevectors where the Fourier amplitude is large. In other words, the phase of a complex number of zero amplitude is undefined. **a**, Topographic image of the $Br_{Te}$ dopant. The white scale bar is 3 nm long. **b**, Map of the amplitude of the 2D-FFT applied to the topographic image. The dashed black circles indicate the position of major peaks in the 2D-FFT and are plot at the same position in the phase maps **de**. **c**, Map of the phase of the 2D-FFT. Because of the phase noise in areas where the amplitude is small, the visualization of the phase pattern is difficult. **d**, Adding dashed white circles around the area where a peak is observed in the amplitude map of the 2D-FFT already helps the visualization of the phase pattern. **e**, To improve even more the visualization, the phase data is only shown within the white dashed circles, otherwise, the phase is set to zero. The same procedure is employed for displaying the phase maps everywhere in the main manuscript and Supplementary. Note that the phase pattern observed here corresponds to the fully symmetry irrep A. For panels **cde**, the white scale bars are equal to the length of the reciprocal lattice vector $\|\vec{a}^\star\|$.

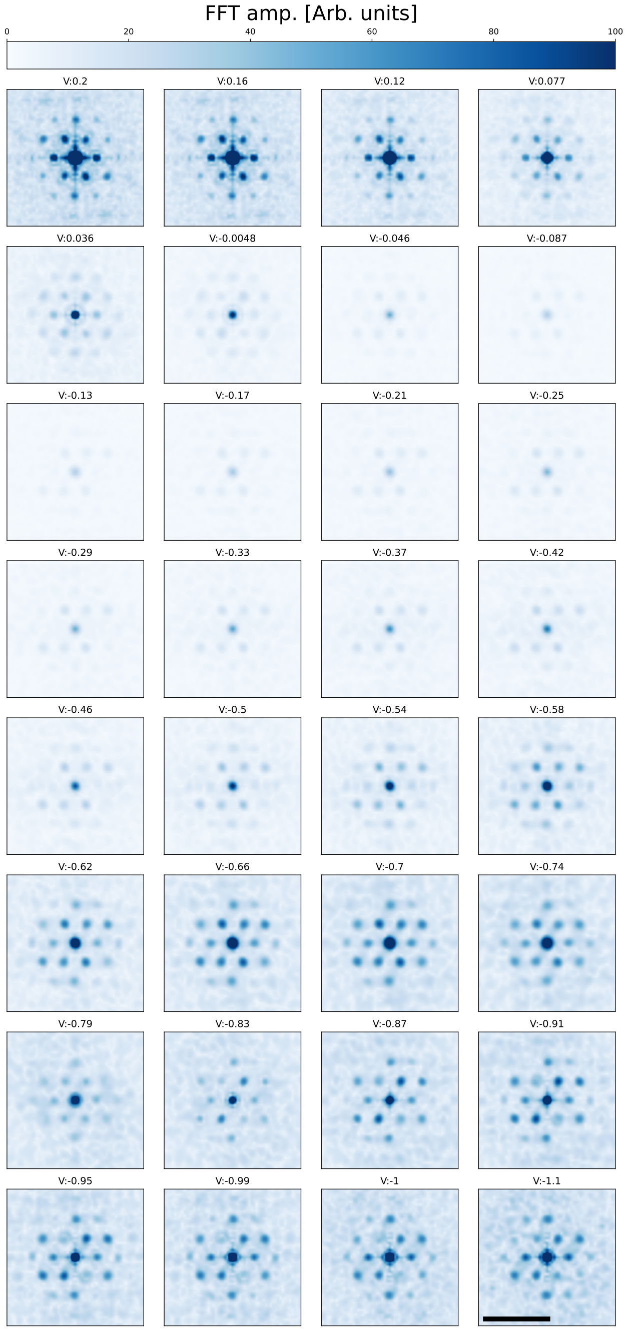


**Fig. 11 Amplitude of 2D-FFT at different sample bias.**. Maps of the amplitude of the 2D-FFT applied to the conductance maps shown in Fig. 9, at different sample bias. The black scale bars show on the last panel is equal to the length of the reciprocal lattice vector $\|\vec{a}^{\star}\|$.

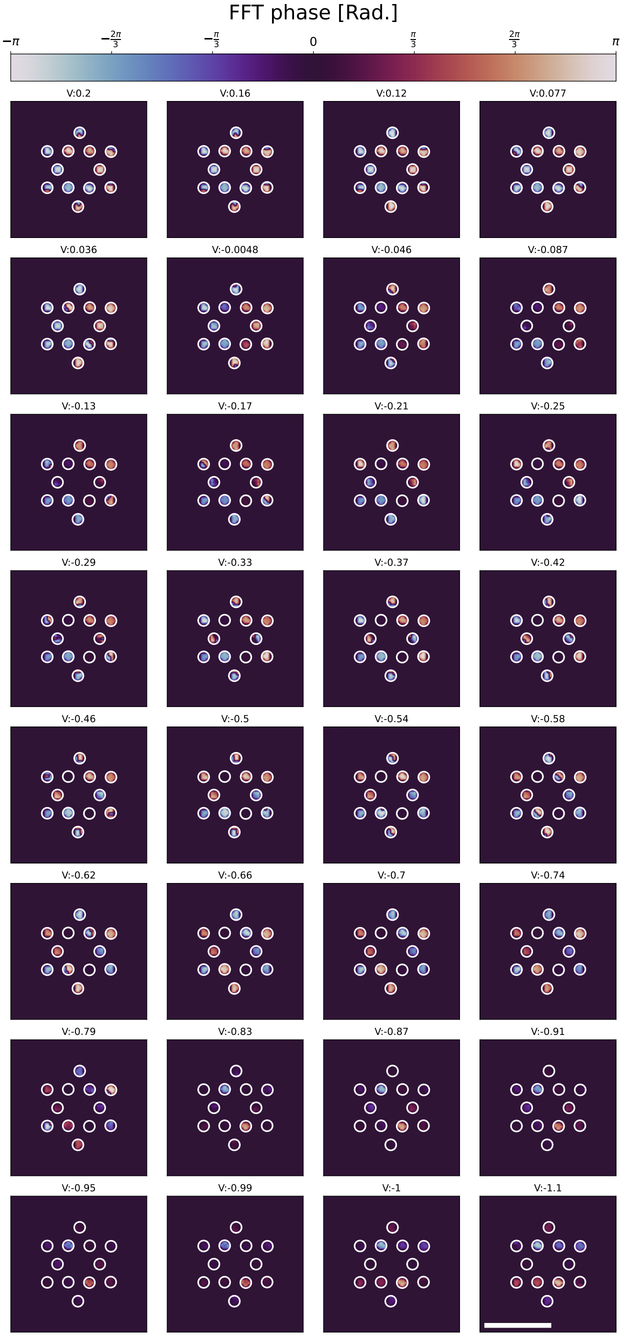


**Fig. 12 Phase of 2D-FFT at different sample bias.**. Maps of the amplitude of the 2D-FFT applied to the conductance maps shown in Fig. 9, at different sample bias. The black scale bars show on the last panel is equal to the length of the reciprocal lattice vector $\|\vec{a}^{\star}\|$.

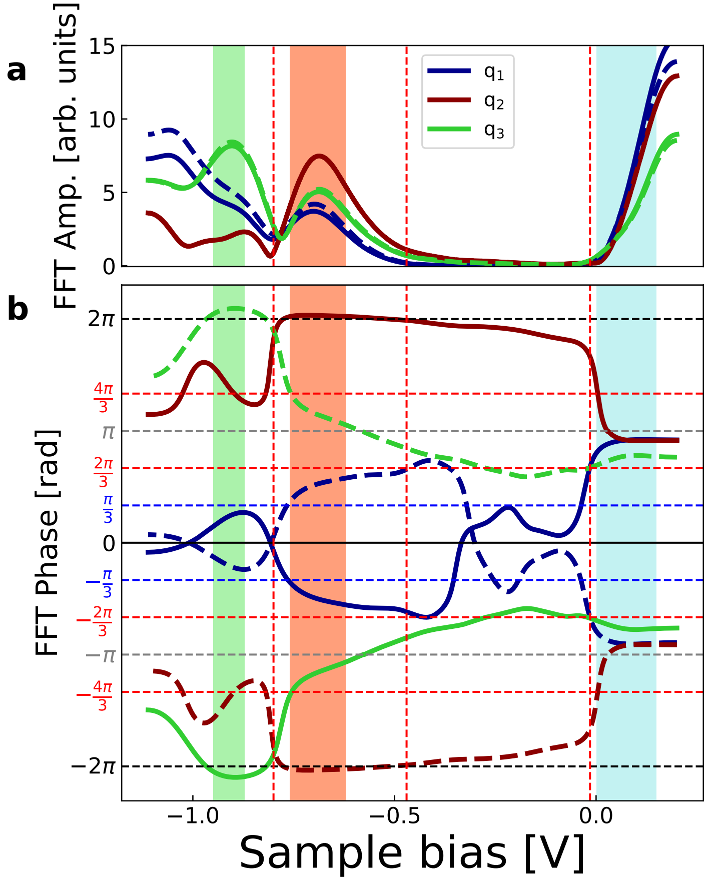


**Fig. 13 Amplitude and phase of the Fourier components $\mathbf{q}_i$. a**, Plot of the amplitude of the Fourier components $q_i$ (continuous line) and $\bar{q}_i$ (dashed line) as function of sample bias. Note the maxima at the sample bias of 0.07 V, -0.7 V and -0.9 V, corresponding to the CBS, IGS and VBS, respectively. **b**, Plot of the phase of the same Fourier components. Note that the phase remains constant in the energy ranges CBS, IGS and VBS, where the phase value is either a multiple of $\pi$ or a multiple of $\pi/3$. Note the rapid phase shift, indicated by vertical red lines, at sample bias -0.015 V, -0.47 V and -0.8 V, separating the CBS from the IGS from the VBS, successively. They indicate change in the symmetry of the dopant states, as expected from the lifting of the valley degeneracy according to the irreps of the double point-group C$_{3\text{v}}$ as shown in Fig. 4a of the main text.

# 6 Side by side comparison of STM maps and theoretical model

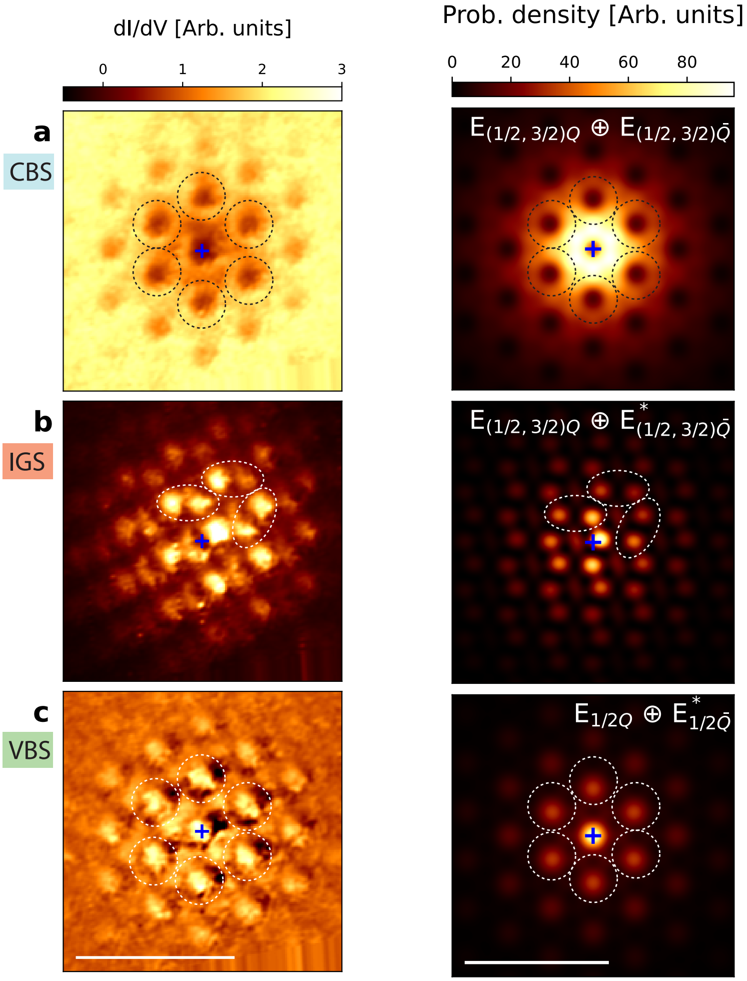


**Fig. 14 Side by side comparison of conductance maps of Br$_{\mathrm{Te}}$ and calculated probability densities. abc**, Conductance maps at sample bias of 0.07 V, -0.7 V and -0.9 V, corresponding to the CBS, IGS and VBS, respectively. The scale bar shown on panel **c** is 3 nm long. **def**, For each panel, the probability density of symmetry adapted eigenstates is calculated for the irrep indicated in the panel. Using the same valley wavevectors, we see that changing the phase factors in the linear combination of valley Bloch states is sufficient to explain the change of spatial maps at different energies. The thin dash lines indicate similar motifs on both the experimental conductance maps and the calculated probability density. As a guide to eye, a plus symbol indicates the center of all images.

# 7 DFT calculations for one MoTe$_2$ monolayer

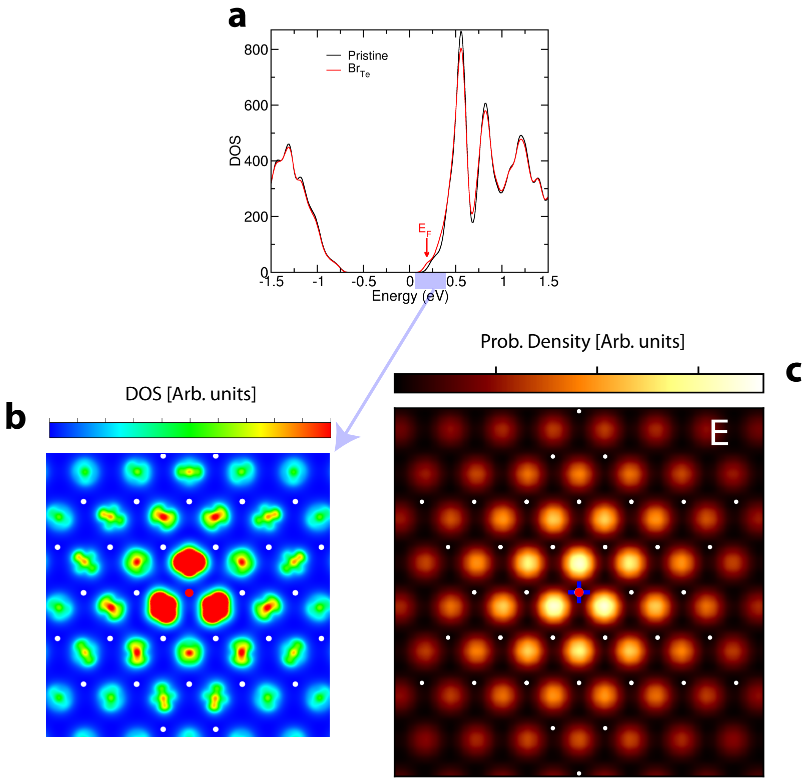


**Fig. 15 DFT calculation of Br$_{\mathrm{Te}}$ dopant in a MoTe$_2$ monolayer. a**, DOS as function of energy for a pristine (black) and Br$_{\mathrm{Te}}$ dopant (red). For the dopant, the DFT calculations show that the last electron-filled state (Fermi energy) is located at the bottom of the conduction band, indicated by a red arrow. **b**, Map of the local DOS, integrated between E$_F$+0.1 V and E$_F$+0.3 V, showing a modulation of the DOS around the dopant. **c**, This modulation is a consequence of the hybridization of the p orbital of the dopant with the Bloch states at the **K**-point of the conduction band, see text. Both images are plot on the same scale. Te atoms are indicated as white dots, the Br atom is indicated as a red dot at the centers of the images.

Density functional theory (DFT) calculations using generalized gradient approximation (GGA) within Perdew-Burke-Ernzerhof parametrization [18] were performed as implemented in the VASP code [19, 20]. A plane-wave cut-off of 450 eV was used in all the calculations. A vacuum space of around 20 Å was considered in the confinement directions to avoid the spurious inter-layer interaction. The full geometry optimizations were performed with the force tolerance being set to 0.02 eV/Å. The Brillouin zone of the studied systems was sampled using 4 x 4 x 1 k-points grid. All the electronic structure calculations

included the spin-orbit coupling (SOC) effect. A 10 x 10 supercell was used for simulations of $Br_{Te}$ substitutions in $MoTe_2$ monolayer. The calculations were limited to one monolayer because of the heavy computational cost of calculating bulk systems.

Because of band structure differences between monolayers and bulk crystals[21], a direct comparison of experimental and DFT data are not possible, however, the DFT results shown Fig. 15 on one monolayer indicate that the dopant levels are also hybridized to the valley Bloch states. They are two major differences with respect to the dopant in the bulk material. First, a plot of the density of states (DOS) as function of energy, Fig. 15a, shows only an impurity level near the conduction band. Second, the spatial modulation of the local DOS, Fig. 15b, indicates that the p orbitals hybridize to the Bloch states at the **K**-point of the conduction band and not to the **Q**-point as observed on the bulk material by STM. As discussed section 1, only the p$_x$,p$_y$-orbitals have contributions to the **K**-points of the conduction band. As these orbitals constitute the basis of the irrep of E symmetry, the dopant level can be described by a wavefunction obtained as a linear combination of Bloch states at the **K**-point adapted to the symmetry of the E irrep. The corresponding probability density is shown Fig. 15c, it has a spatial modulation compatible with the DFT results. In particular, note the minima of DOS at the impurity site; furthermore, on the DOS map calculated by DFT, note also that each local maxima has a complex structure that cannot be described by the simple Bloch model.

The absence of impurity level within the band gap, near the valence band, is not clearly understood but should be the consequence of different screening and different hybridization properties, **K**-point vs **Q**-point, between the monolayer and bulk materials.

Finally, Fig. 16 shows the partial density of states (PDOS) as function of energy for the p-orbitals and d-orbitals of the Br atom and the p and d orbitals of the 1st and 2nd neighbors Mo atoms surrounding the Br atom. We see that near zero energy, where is located the donor-state, a large contribution arise from the p$_x$+p$_y$ orbitals of the Br atom but the largest contribution arise from the d$_{z^2}$ orbitals of the 1st and 2nd neighbors Mo atoms. As it is well established that the Bloch states at the **K**-point have $d_{z^2}$ character, this confirms the hybridization of the dopant p-orbitals with the Bloch states of the conduction band at the **K**-valleys.

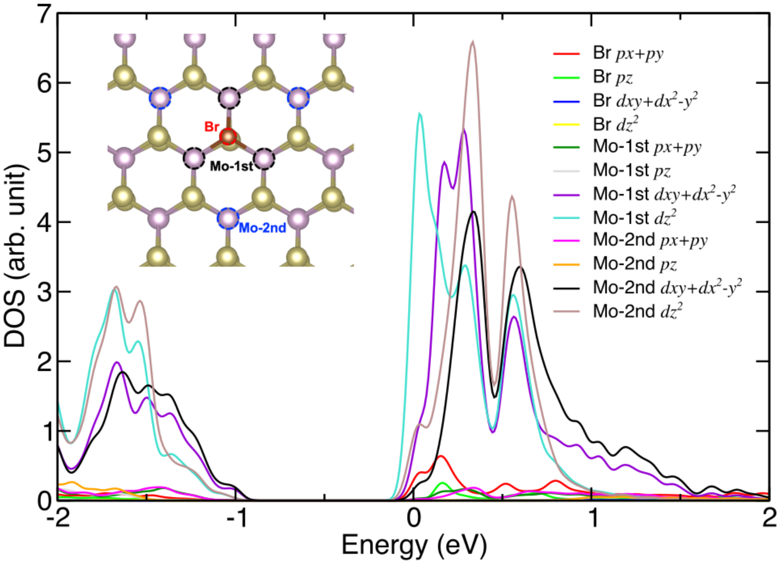


**Fig. 16 Partial density of states for $Br_{Te}$ dopant in a $MoTe_2$ monolayer.** From the DFT calculations, we extract the PDOS as function of energy for the p-orbitals and d-orbitals of the Br atom and the p- and d-orbitals of the 1st and 2nd neighbors Mo atoms surrounding the Br atom. We see that near zero energy, where is located the donor-state, a large contribution arise from the $p_x$+$p_y$ orbitals of the Br atom but the largest contribution arise from the $d_{z^2}$ orbitals of the 1st and 2nd neighbors Mo atoms. This is consistent with expected E symmetry of the Bloch states at the **K**-point and confirm the hybridization of the dopant level with the Bloch states at the **K**-valleys known to have mostly $d_{z^2}$ character.

# References

[1] Kohn, W., Luttinger, J.M.: Theory of donor states in silicon. Phys. Rev. **98**(4), 915–922 (1955)

[2] Evarestov, R.A., Smirnov, V.P.: Application of band representations of space groups in the theory of phase transitions and point defects in crystals. Phys. Status Solidi B Basic Res. **136**(2), 409–415 (1986)

[3] Bradlyn, B., Elcoro, L., Cano, J., Vergniory, M.G., Wang, Z., Felser, C., Aroyo, M.I., Bernevig, B.A.: Topological quantum chemistry. Nature **547**(7663), 298–305 (2017)

[4] Aroyo, M.I., Perez-Mato, J.M., Capillas, C., Kroumova, E., Ivantchev, S., Madariaga, G., Kirov, A., Wondratschek, H.: Bilbao crystallographic server: I. databases and crystallographic computing programs. Zeitschrift für Kristallographie - Crystalline Materials **221**(1), 15–27 (2006)

[5] Elcoro, L., Bradlyn, B., Wang, Z., Vergniory, M.G., Cano, J., Felser, C., Bernevig, B.A., Orobengoa, D., de la Flor, G., Aroyo, M.I.: Double crystallographic groups and their representations on the bilbao crystallographic server. J. Appl. Crystallogr. **50**(5), 1457–1477 (2017)

[6] Liu, G.-B., Xiao, D., Yao, Y., Xu, X., Yao, W.: Electronic structures and theoretical modelling of two-dimensional group-VIB transition metal dichalcogenides. Chem. Soc. Rev. **44**(9), 2643–2663 (2015)

[7] Bradley, C., Cracknell, A.: The Mathematical Theory of Symmetry in Solids: Representation Theory for Point Groups and Space Groups. Oxford University Press, ??? (2010)

[8] Shklovskii, B.I., Efros, A.: Electronic Properties of Doped Semiconductors, p. 388. Springer, ??? (1984)

[9] Title, R.S., Shafer, M.W.: Electron-Paramagnetic-Resonance studies on arsenic acceptors in natural (2h) and synthetic (3r) MoS$_2$ crystals. Phys. Rev. B Condens. Matter **8**(2), 615–620 (1973)

[10] Stone, N.J.: Table of nuclear electric quadrupole moments. At. Data Nucl. Data Tables **111-112**, 1–28 (2016)

[11] Stoll, S., Schweiger, A.: EasySpin, a comprehensive software package for spectral simulation and analysis in EPR. J. Magn. Reson. **178**(1), 42–55 (2006)

[12] Stopkowicz, S., Cheng, L., Harding, M.E., Puzzarini, C., Gauss, J.: The bromine nuclear quadrupole moment revisited. Mol. Phys. **111**(9-11),

1382–1389 (2013)

[13] Bettin, Knöckel, Tiemann: Hyperfine structure measurements in the B3IIo+ u—x 1Σ+ g electronic transition of br2. Chem. Phys. Lett. (1981)

[14] Haas, H., Petrilli, H.M.: Quadrupole moments of the halogen nuclei. Phys. Rev. B Condens. Matter **61**(20), 13588–13592 (2000)

[15] Merkulov, I.A., Efros, A.L., Rosen, M.: Electron spin relaxation by nuclei in semiconductor quantum dots. Phys. Rev. B Condens. Matter **65**(20), 205309 (2002)

[16] Jiang, M., Wu, Z., Yang, Q., Zhang, Y., Men, Y., Jia, T., Sun, Z., Feng, D.: Coherent spin dynamics of localized electrons in monolayer MoS2. J. Phys. Chem. Lett. **13**(11), 2661–2667 (2022)

[17] Wu, Y., Tong, Q., Liu, G.-B., Yu, H., Yao, W.: Spin-valley qubit in nanostructures of monolayer semiconductors: Optical control and hyperfine interaction. Phys. Rev. B Condens. Matter **93**(4), 045313 (2016)

[18] Perdew, J.P., Burke, K., Ernzerhof, M.: Generalized gradient approximation made simple. Phys. Rev. Lett. **77**(18), 3865–3868 (1996)

[19] Kresse, G., Furthmüller, J.: Efficient iterative schemes for ab initio total-energy calculations using a plane-wave basis set. Phys. Rev. B Condens. Matter **54**(16), 11169–11186 (1996)

[20] Kresse, G., Joubert, D.: From ultrasoft pseudopotentials to the projector augmented-wave method. Phys. Rev. B Condens. Matter **59**(3), 1758–1775 (1999)

[21] Splendiani, A., Sun, L., Zhang, Y., Li, T., Kim, J., Chim, C.-Y., Galli, G., Wang, F.: Emerging photoluminescence in monolayer MoS2. Nano Lett. **10**(4), 1271–1275 (2010)
